# Supplementary material for: Interplay of Mechanochemistry and Material Processes in the Graphite to Diamond Phase Transformation
Source: arXiv:2302.04684 source file (2023-02-09)
Supplement: Supplementary file 1 [file Graphite_Supplemental_Materials.pdf]

# Supplemental Materials to:
# Interplay of Mechanochemistry and Material Processes in the Graphite to Diamond Phase Transformation

Brenden W. Hamilton, Timothy C. Germann
Theoretical Division, Los Alamos National Laboratory, Los Alamos, New Mexico 87545, USA

## SM-1

Within the framework of the LAMMPS software package, MBsMD utilizes explicit bonding to define the steered MD system. In this case, a network of improper dihedrals is pre-defined in the atomic configuration data file. All atoms are fully described by the ReaxFF forcefield, and those within any of the improper groups also have an energy contribution from a harmonic function based on the out of plane angle of the improper dihedral. For a given, the minimum energy point on the potential is set to be the same out of plane angle for all improper groups and ranges from 0 to 50 degrees, by 10-degree jumps.

In order to prevent the external potential from influencing the direction of dynamics after the graphite layers begin to break up and/or react, each improper has a variable setting to be turned on or off. In the LAMMPS framework, this is done using the 'delete_bonds' command, which will remove any individual bonding topology group from active service, but it will continue to store that it exists.

To determine whether or not an improper should be influencing the system, we use the ReaxFF bonding environments. ReaxFF stores a 'bond table' every N steps. This table lists, for each atom, all other atoms it is currently bonded to, known as its bonding environment. The bonding environment for all atoms in an improper dihedral is stored at step zero. Every 0.1 ps, the current bonding environment for those atoms is compared to their initial bonding environment. For impropers with any of its 4 atoms that differs, it is turned off. Those with identical to initial bonding environments continue to feel the external field to deform out of plane. Additionally, any improper that is currently turned off that returns to its original bonding environment will be turned back on.

Little to no improper groups a deactivated prior to phase transformation, and all groups are turned off by the time transformation is complete. This prevents the external field from imposing some local deformation within the diamond lattice that could induce defect formation or cause a polyhedral template matching algorithm to misidentify the local structure.

## SM-2

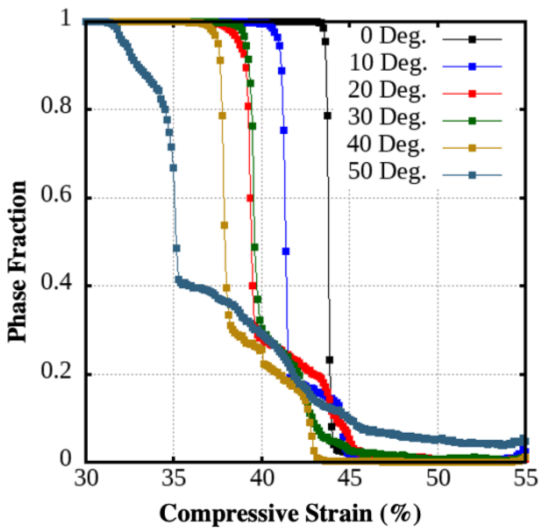

SM Figure 1: Graphite population histories for different out of plane strain values.

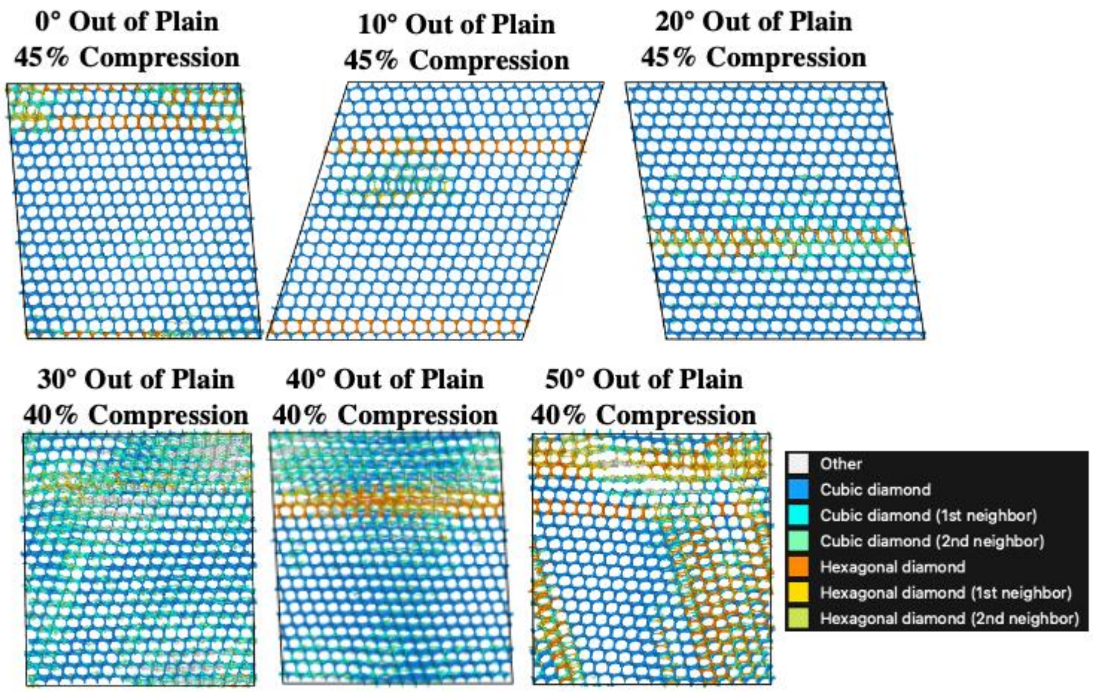

SM Figure 2: Atomic rendering of defect formations during graphite to diamond phase transformations for each out of plane strain.

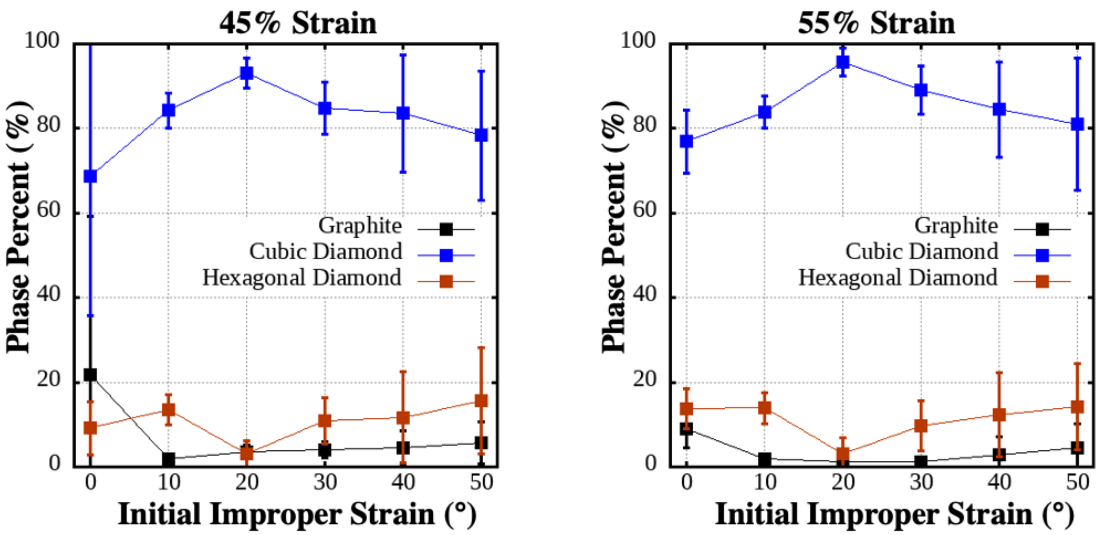


SM Figure 3: Summary phase amounts figure, mirroring manuscript Figure 4, for different compressive strain levels.
